# Supplementary material for: Topological Separation of Vortices
Source: arXiv:2407.03384 ancillary file (2024-12-17)
Supplement: Supplementary file 1 [file supp_doc.pdf]

# Topological Separation of Vortices: Supplemental Document

Adeel Zafar\*

Zahra Poorshayegh†

Di Yang‡

Guoning Chen§

University of Houston

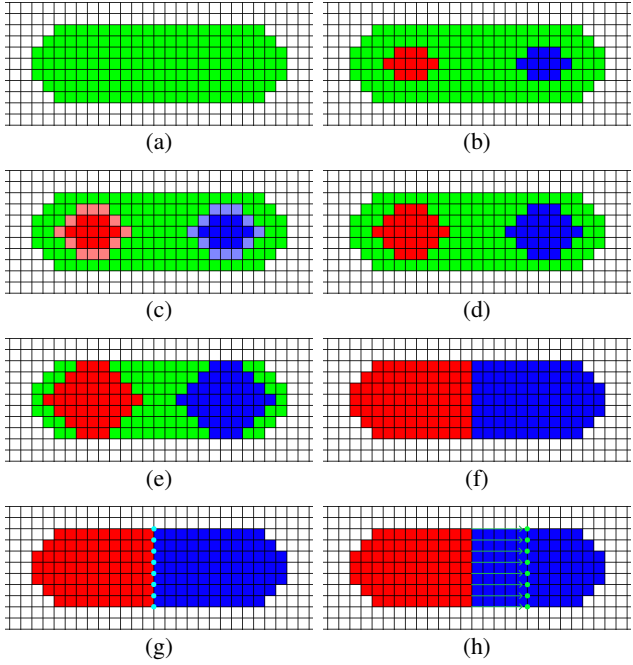

Figure 1: This figure illustrates the splitting process of a vortical region using a 2D grid for ease of explanation. (a) shows a vortical region (green). (b) shows the initial contour tree-based segmentation in the form of the query segment (green) and seed segments (red and blue). (c) and (d) show one iteration of the layering. (c) shows the immediate neighboring cells (light red and light blue) of the seed segments in the query segment. (d) shows the end of the first iteration. (e) shows the end of the second iteration. (f) shows the final iteration of the layering where no cells are left in the query segment. (g) shows the boundary points (cyan). (h) shows the seed points (green) to compute vorticity lines which are five layers of cells away from the boundary points towards the bigger region.

## 1 ADDITIONAL DETAILS

In the following, we provide additional details for the methods discussed, such as Region Growing [1], Splitting, and Layering. Fig. 1(a) shows a vortical region. Using, e.g.,  $\lambda_2$ , the vortical regions are extracted by finding the unstructured grids where the points fulfill the criterion that  $\lambda_2 < 0$ . However, in practice,  $\lambda_2 < 0$  is less strict. In Region Growing [1], we statistically find a threshold  $\lambda_{2i}$  such that  $\lambda_2 < \lambda_{2i}$ , which is practically more stable. In Fig. 1(b), the red and blue segments, and the green segment correspond to the two minima and maximum, respectively, of the minimal join tree-

\*e-mail: azafar3@uh.edu

†e-mail: zpoorsha@uh.edu

‡e-mail: diyang@uh.edu

§e-mail: gchen16@uh.edu

## Algorithm 1 Vortex Separation Algorithm

---

```

procedure GET_SEGMENTS(vortexData)
  → Get critical point pairs with the highest persistence.
  → Perform topological simplification of vortexData.
  → segmentIds ← Extract join tree and get segmentation.
  * segmentIds holds the segment ids for each cell

return segmentIds
end procedure

procedure LAYER(segmentIds, querySegment, seedSegments)
  → cellIds ← neighbors of seedSegments in querySegment.
  → Update segmentIds of cellIds.
end procedure

procedure FIX_SEGMENTS(vortexData, segmentIds)
  → querySegment ← cells with the segmentIds = -1.
  → seedSegments ← cells with the segmentIds ≠ -1.
  → N ← Number of cells in querySegment
  while N ≠ 0 do
    → LAYER(segmentIds, querySegment, seedSegments)
  end while
return segmentIds
end procedure

procedure AVOID_SPLIT(vortexData, segmentIds)
  → Find boundary points between the two segments.
  → Find seed points slightly away from the boundary points.
  → Extract streamlines using the vorticity vector field.
  → R1 = # of cells overlapped by streamlines in segment 1.
  if R1 ≥ 0.25 then
    return true
  else
    return false
  end if
end procedure

procedure SEPARATE(vortexData, regionIds)
  N ← 0
  while N < 2 do
    → segmentIds ← GET_SEGMENTS(vortexData)
    → segmentIds ← FIX_SEGMENTS(vortexData, segmentIds)
    → N ← Number of unique ids in segmentIds
    → avoidSplit ← AVOID_SPLIT(vortexData, segmentIds)
    if avoidSplit then
      continue
    end if
  end while
  → Update regionIds with segmentIds.
  → Get newVortices[ ] from vortexData using segmentIds.
  for newVortex in newVortices do
    → SEPARATE(newVortex, regionIds)
  end for
end procedure

procedure MAIN(inputDataset)
  → Use Region_growing() from [1] to get vortexRegions.
  → Initialize regionIds
  * regionIds array keeps track of the vortex hierarchy
  for disconnectedRegion in vortexRegions do
    → SEPARATE(disconnectedRegion, regionIds)
    * Begin separation for each disconnected region
  end for
end procedure

```

---

based segmentation explained in Section 3.1 of the main paper. The subsequent steps of the layering process are shown in Fig. 1(c, d, e, f), respectively.

Table 1: This table shows the performance statistics (*in minutes(m)*) of the flow datasets used in our experiments. *Segmentation Time* shows the performance of obtaining the initial contour tree-based segmentation. *Layering Time* shows the time it takes to perform the layering. *Avoid Split Time* is the time it takes to find the optimal seeds, extract vorticity lines, and decide whether to avoid the split. *PP Time* is the time it takes for post-processing (PP) steps, including thresholding the new regions and recording the changes in the vortex hierarchy. *Total Time* is the total time taken for the complete splitting process of the whole dataset. The performance is measured on a PC with an Intel Xeon(R) CPU E5-2640 without multiprocessing.

| Data Set     | #Points | #Cells  | Performance           |                   |                      |             |                |
|--------------|---------|---------|-----------------------|-------------------|----------------------|-------------|----------------|
|              |         |         | Segmentation Time (m) | Layering Time (m) | Avoid Split Time (m) | PP Time (m) | Total Time (m) |
| Couette Flow | 2169086 | 1580627 | 78                    | 110               | 891                  | 14          | 229            |
| Channel Flow | 2476391 | 1570420 | 250                   | 454               | 19                   | 37          | 787            |

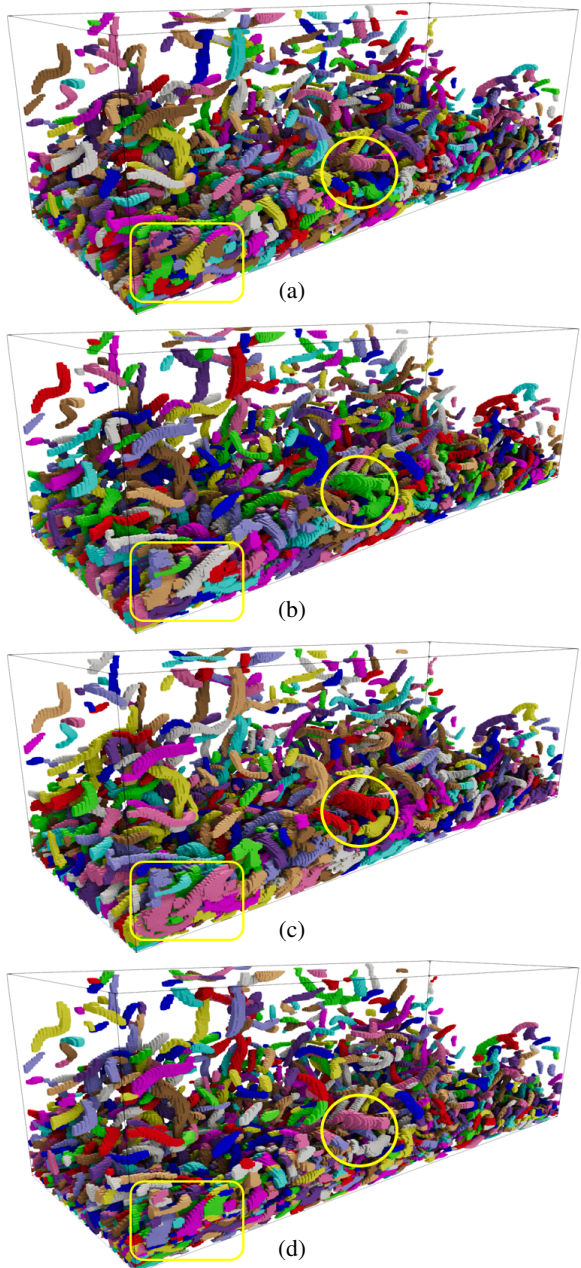

Figure 2: (a) Zoomed in views of Fig. 9 (b, c, d, e) from the main text.

## 2 PSEUDO-CODE FOR VORTEX SEPARATION

The pseudo-code for the method is given in [Algorithm 1](#). The algorithm starts with the MAIN function, where we first extract the vortical regions using the Region Growing approach [1]. *regionIds* is an array that keeps track of the region id assigned to each cell. For each separate vortical region, we call the SEPARATE procedure. The parameter *vortexData* represents the vortical region. In the SEPARATE procedure, we set  $N=0$ , where  $N$  is an integer which stores the number of new regions. The splitting process is done inside the **while** loop. We first get the initial contour tree-based segmentation using the GET\_SEGMENTS function. Then we call the FIX\_SEGMENTS function, which performs the layering process and splits the region into two new regions as illustrated in [Fig. 1](#). We store the number of new regions in the variable  $N$ . Then we call the AVOID\_SPLIT function that checks and decides if the region should be split or not. If 'Yes', the **while** loop ends and we record the changes in *regionIds* and continue the recursive process on the new regions. If 'No', the next iteration of the loop starts, where the GET\_SEGMENTS function chooses the next (minimum-saddle) pair with the highest persistence. If we have exhausted all the (minimum-saddle) pairs, then the **while** loop ends, terminating the process for the current region.

## 3 ADDITIONAL RESULTS

[Fig. 2](#) shows the zoomed-in views of the vortex separation results on the channel flow dataset from [Fig. 9](#) of the main paper. [Tab. 1](#) shows the performance of the algorithm in the current implementation of the method. We will improve this implementation to make it practical for large-scale datasets.

## ACKNOWLEDGMENTS

We thank the anonymous reviewers for their valuable feedback. This research was supported by NSF OAC 2102761.

## REFERENCES

- [1] A. Zafar, D. Yang, and G. Chen. Extract and characterize hairpin vortices in turbulent flows. *IEEE Transactions on Visualization and Computer Graphics*, 30(1):716–726, 2024. doi: 10.1109/TVCG.2023.3326603 1, 2
